# Supplementary material for: Demonstration-Regularized RL
Source: arXiv:2310.17303 source file (2024-06-10)
Supplement: Supplementary file 1 [file Regularised-MDP.tex]

\section{Regularized MDPs}\label{app:regularized_mdp}

In this section we describe the general setting of regularized MDPs, not only entropy-regularized.

\subsection{Preliminaries}
\todoPi{Maybe keep only the $\KL$ to keep things simple for the reader? }

First we define class of regularizers we are interested in. For more exposition on this definition, see \cite{bubeck2015convex}. 
\begin{definition}\label{def:mirror_map}
    Let $\Phi \colon \simplex_{\cA} \to \R$ be a proper closed strongly-convex function. We will call $\Phi$ a mirror-map if the following holds 
\begin{itemize}
    \item $\Phi$ is $1$-strongly convex with respect to norm $\norm{\cdot}$;
    \item $\nabla \Phi$ takes all possible values in $\R^{\cA}$;
    \item $\nabla \Phi$ diverges on the boundary of $\simplex_{\cA}$: $\lim_{x \in \partial \simplex_{\cA}} \norm{\nabla \Phi(x)} = +\infty$;
\end{itemize}
\end{definition}

As a regularizer, we will allow $\Phi$ be different for each $h$ and $s$, as in the main example
\[
    \Phi_{h,s}(\pi) = \KL(\pi \Vert \pi^{\base}_h(s)),
\]
where $\pi^\base \in \simplex_A^{H \times S}$ is a fixed policy.

Next we define a convex conjugate to $\lambda \Phi_{h,s}$ as $F_{\lambda,h,s} \colon \R^{\cA} \to \R$
\[
    F_{\lambda,h,s} (x) = \max_{\pi \in \simplex_{\cA}} \{ \langle \pi, x \rangle - \lambda \Phi_{h,s}(\pi) \}
\]
and, with a sight abuse of notation extend the action of this function to the $Q$-function as follows
\[
    \Vstar_{\lambda,h}(s) = F_{\lambda,h,s}(\Qstar_{\lambda,h})(s) = \max_{\pi \in \Delta_{\cA}}\left\{ \pi \Qstar_{\lambda,h}(s) - \lambda \Phi_{h,s}(\pi) \right\}.
\]

Thanks to the fact that $\Phi_{h,s}$ satisfies Definition~\ref{def:mirror_map}, we have exact formula for the optimal policy by Fenchel-Legendre transform
\[
    \pi^\star_h(s) = \argmax_{\pi \in \Delta_{\cA}}\left\{ \pi \Qstar_{\lambda,h}(s) - \lambda \Phi_{h,s}(\pi) \right\} = \nabla F_{\lambda,h,s}(\Qstar_{\lambda,h}(s,\cdot)).
\]
Notice that we have $\nabla F_{\lambda,h,s}(\Qstar_{\lambda,h}(s,\cdot)) \in \simplex_{\cA}$ since the gradient of $\Phi$ diverges on the boundary of $\simplex_{\cA}$. For entropy regularization this formula become the softmax function, and for KL-divergence this formula becomes exponential weights formula.

Finally, it is known that the smoothness property of $F_{\lambda,h,s}$ plays a key role in reduced sample complexity for planning in regularized MDPs \cite{grill2019planning}. For our general setting we have that since $\lambda \Phi_{h,s}$ is $\lambda$-strongly convex with respect to $\norm{\cdot}$, then $F_{\lambda}$ is $1/\lambda$-strongly smooth with respect to a dual norm $\norm{\cdot}_*$
\[
    F_{\lambda,h,s}(x) \leq F_{\lambda,h,s}(x') + \langle \nabla F_{\lambda,h,s}(x'), x-x' \rangle + \frac{1}{2\lambda} \norm{x - x'}_*^2.
\]
We assume that $\Phi \geq 0$ and $\Vstar_{\lambda, h}(s) \geq 0$ for any $s$. This condition is satisfied in the example of KL-divergence, however, we do not restrict our assumption to KL-divergence. It could be any divergence with respect to any fixed policy.

Also, since all norms in $\R^\cA$ are equivalent, we define a constant $r_A$ that defined for a dual norm $\norm{\cdot}_*$ as follows
\[
    \norm{\cdot }_* \leq r_A \cdot \norm{\cdot}_\infty.
\]
For example, for $\ell_2$-norm $r_A = \sqrt{A}$ and for $\ell_1$-norm $r_A = A$. In the case $\Phi = -\cH$ we have $r_A = 1$ since the entropy is $1$-strongly convex with respect to a $\ell_1$-norm, thus the dual norm is exactly a $\ell_\infty$-norm.
